# Supplementary material for: Attractor Memory for Long-Term Time Series Forecasting: A Chaos Perspective
Source: arXiv:2402.11463 source file (2024-11-02)
Supplement: Supplementary file 1 [file 6.Appendix.tex]

% \appendix
% \onecolumn

% \renewcommand{\cftsecfont}{\normalfont\bfseries}
% \begin{center}
%     \Large{\sc\Huge Supplementary material\\\large Attractor Memory for Long-Term \\Time Series Forecasting: A Chaos Perspective}\\
% \end{center}
% \vskip 4mm
% \startcontents[sections]\vbox{\sc\Large Table of Contents}
% %\vspace{5mm}
% \hrule height .8pt
% %\vspace{-2mm}
% \printcontents[sections]{l}{1}{\setcounter{tocdepth}{2}}
% %\vspace{4mm}
% \hrule height .8pt
% \vskip 10mm
% % \clearpage

% \input{icml2024/appendix_list/a_technical}
% \input{icml2024/appendix_list/b_model}
% \input{icml2024/appendix_list/c_exp}
